# Supplementary material for: Frugal Optimization for Cost-related Hyperparameters
Source: arXiv:2005.01571 source file (2020-12-22)
Supplement: Supplementary file 1 [file sec_appendix_ceo_normalization.tex]

\section{\HPOname with Search Space Normalization}

\begin{algorithm}[h]
\caption{\HPOname (with normalization)}\label{alg:hpo_normalized}
\begin{algorithmic}[1]
\State \textbf{Inputs:} 1. Normalized feasible search space $\cX$, the dimensionality of which is $d$. 2. Initial low-cost configuration $\bx_0$.
\State \textbf{Initialization:} Set initial value $\bx = \bx_0$
(and get $f(\bx)$), $\delta = \delta_{init}$, $k = k'= n = r =0$, $l^{\text{r-best}} = +\text{inf}$
\While{Budget allows} 
    \State Sample $\bu$ uniformly at random from $\bbS$
    % \State $\bx^{+}  \gets \bx + \delta \bu $, $\bx^{-} \gets  \bx - \delta \bu$
    \State $\bx^{+} \gets \Proj_{\cX}(\bx + \delta \bu)$, $\bx^{-} \gets \Proj_{\cX}(\bx - \delta \bu)$
    \If{$f(\bx^{+}) < f(\bx)$}
        $\bx \gets \bx^{+}$ %and report $\bx$
        %$\Proj_{\cC}(\tS(e^{\bx_{k+1}}))$
    \ElsIf{$f(\bx^{-}) < f(\bx)$}
            $\bx \gets \bx^{-}$ %and report $\bx$
            % the model trained with 
            %$\Proj_{\cC}(\tS(e^{\bx_{k+1}}))$
        \Else
            \space $n \gets n +1$
    \EndIf
   
     \If{$f(\bx) < l^{\text{r-best}}$}             $l^{\text{r-best}} \gets f(\bx) $ and $ k' \gets k$  
    \EndIf
    \State $k \gets k+1$
    \If{$n=2^{d-1}$}
      % \State $K_{\text{old}} \gets k'' - k'$ if $K_{\text{new}} = 0$, else $K_{\text{old}} \gets K_{\text{new}}$
        \State $n\gets 0$, $\delta \gets \delta \frac{1}{\sqrt{\eta}}, $ in which $\eta = \frac{k}{k'}$
        \If{$\delta \leq \delta_{\text{lower}}$ }
            \State $k \gets 0$, $l^{\text{r-best}} \gets +\text{inf}$
            \State Reset $\bx \gets \mathbf{g}$, where $\mathbf{g} \sim N(\bx_0, \mathbf{I})$  %Reset config
            \State $ r\gets r+1$ and $\delta \gets r + \delta_{init}$
        \EndIf
  \EndIf
\EndWhile
\end{algorithmic}
\end{algorithm}
